# Supplementary material for: DualDiff: Dual-branch Diffusion Model for Autonomous Driving with Semantic Fusion
Source: arXiv:2505.01857 source file (2025-05-03)
Supplement: Supplementary file 1 [file appendix.tex]

\appendix
\section{Object Filtering}
\begin{figure}[ht]
    \centering
    \includegraphics[width=0.98\linewidth]{figure/box_and_view2}
    \caption{Bounding box filtering to each view. The dashed lines in (b-c) represent the $x$-axis of the camera's coordinates. Boxes are retained only if they have at least a point in the positive half of the $z$-axis in each camera's coordinate.}
    \label{fig:visible_box}
    \vspace{-0.2cm}
\end{figure}

In \Eqref{equ:box_filter}, 
we employ $f_{viz}$ for object filtering to facilitate bootstrap learning. We show more details of $f_{viz}$ here. Refer to \Figref{fig:visible_box} for illustration.
For the sake of simplicity, each camera's Field Of View (FOV) is not considered. Objects are defined as \textit{visible} if any corner of their bounding boxes is located in front of the camera (\ie, $z^{v_{i}}>0$) within each camera’s coordinate system. The application of $f_{viz}$ significantly lightens the workload of the bounding box encoder, evidence for which can be found in 
\Secref{sec:ablation}.

\section{More Experimental Details}\label{app:exp_setup}
\textbf{Semantic Classes for Generation.}
To support most perception models on nuScenes, we try to include semantics commonly used in most settings~\citep{huang2021bevdet,zhou2022cross,liu2022bevfusion,ge2023metabev}.
Specifically, for objects, ten categories include car, bus, truck, trailer, motorcycle, bicycle, construction vehicle, pedestrian, barrier, and traffic cone.
For the road map, eight categories include drivable area, pedestrian crossing, walkway, stop line, car parking area, road divider, lane divider, and roadblock.

\textbf{Optimization.}
We train all newly added parameters using AdamW~\citep{loshchilov2018decoupled} optimizer and a constant learning rate at $8e^{-5}$ and batch size 24 (total 144 images for 6 views) with a linear warm-up of 3000 iterations, and set $\gamma^{s}=0.2$.

\section{Ablation on Number of Attending Views}\label{app:ablation_view}
\input{tables/attention-number}
\begin{figure}[t]
    \vspace{-0.3cm}
    \centering
    \includegraphics[width=\linewidth]{figure/attend_views}
    \vspace{-0.2cm}
    \caption{{Comparison between different numbers of attending views.} Only attending to one view results in worse multi-camera consistency.}
    \label{fig:attending-views}
    \vspace{-0.2cm}
\end{figure}
In \Tabref{tab:attend_ablation}, we demonstrate the impact of varying the number of attended views on evaluation results.
Attending to a single view yields superior FID results; the reduced influx of information from neighboring views simplifies optimization for that view.
However, this approach compromises mIoU, also reflecting less consistent generation, as depicted in \Figref{fig:attending-views}.
Conversely, incorporating all views deteriorates performance across all metrics, potentially due to excessive information causing interference in cross-attention.
Since each view has an intersection with both left and right views, attending to one view cannot guarantee consistency, especially for foreground objects, while attending to more views requires more computation.
Thus, we opt for 2 attended views in our main paper, striking a balance between consistency and computational efficiency.

\section{Qualitative Comparison with BEVGen}\label{sec:comp-bevgen}
\Figref{fig:comparison-bevgen} illustrates that \methodname generates images with higher quality compared to BEVGen~\citep{swerdlow2023street}, particularly excelling in objects.
Such enhancement can be attributed to \methodname's utilization of the diffusion model and the adoption of a customized condition injection strategy. 

\begin{figure}[h]
    \centering
    \includegraphics[width=0.98\linewidth]{figure/comparison_bevgen.pdf}
    \caption{Qualitative comparison with BEVGen on driving scene from nuScenes validation set. We highlight some areas with rectangles to ease comparison. Compared with BEVGen, image quality of objects from \methodname is much better.
    }
    \label{fig:comparison-bevgen}
    \vspace{-0.5cm}
\end{figure}

\section{More results with control from different conditions}\label{sec:scene-level}
\Figref{fig:scene-level} shows \textit{scene level} control (time of day) and \textit{background level} control (BEV map alterations). \methodname can effectively reflect these changes in control conditions through the generated camera views.

\begin{figure}[h]
    \centering
    \includegraphics[width=0.98\linewidth]{figure/main_results2.2}
    \caption{Showcase for scene-level control with \methodname. The scene is from the nuScenes validation set.}
    \label{fig:scene-level}
\end{figure}

\newpage
\section{More Experiments with 3D Object Detection}
\input{tables/bevfusion_train}
In \Tabref{tab:bevfusion_train_full}, we show additional experimental results on training 3D object detection models using synthetic data produced by \methodname. Given that BEVFusion utilizes a lightweight backbone (\ie, Swin-T~\citep{liu2021Swin}), model performance appears to plateau with training through 1-2$\times$ epochs (2$\times$: 20 for CAM-Only and 6 for CAM+LiDAR). Reducing epochs can mitigate this saturation, allowing more varied data to enhance the model's perceptual capacity in both settings. This improvement is evident even when epochs for 3D object detection are further reduced to 0.5$\times$. Our \methodname accurately augments street-view images with the annotations.
Future works may focus on annotation sampling and construction strategies for synthetic data augmentation.

\section{More Discussion}
\paragraph{More future work.}
Note that \methodname-generated street views can currently only perform as augmented samples to train with real data, and it is exciting to train detectors solely with generated data, which will be explored in the future.
More flexible usage of the generated street views beyond data augmentation, especially incorporation with generative pre-training~\citep{chen2023mixed,zhili2023task}, contrastive learning~\citep{chen2021multisiam,liu2022task} and the large language models (LLMs)~\citep{chen2023gaining,gou2023mixture}, is an appealing future research direction.
It is also interesting to utilize the geometric controls in different circumstances beyond 3D scenarios (\eg, multi-object tracking~\citep{li2023trackdiffusion} and concept removal~\citep{liu2023geomerasing}).

\section{Detailed Analysis on 3D Object Detection with Synthetic Data}

\begin{table}[h]
\setlength{\tabcolsep}{2.2pt}
\centering
\caption{Per-class performance comparison with BEVFusion for 3D object detection with $1\times$ setting. Results are tested on the nuScenes validation set.}
\label{tab:bevfusion_compare}
\begin{tabular}{l|c|cccccccccc}
\toprule
Data         & mAP   & car   & cone  & barrier & bus   & ped. & motor. & truck & bicycle & trailer & constr. \\
\midrule
BEVFusion & 32.88 & 50.67 & 50.46 & 48.62   & 37.73 & 35.74      & 30.40      & 27.54 & 24.85   & 15.56   & 7.28         \\
$+$ \methodname  & 35.40 & 51.86 & 53.56 & 51.15   & 40.43 & 38.10      & 33.11      & 29.35 & 27.85   & 18.74   & 9.83         \\
\midrule
Difference      &
\textcolor{green}{+2.52}  &
\textcolor{green}{+1.20}  &
\textcolor{green}{+3.10}  &
\textcolor{green}{+2.53}  &
\textcolor{green}{+2.70}  &
\textcolor{green}{+2.36}  &
\textcolor{green}{+2.71}  &
\textcolor{green}{+1.81}  &
\textcolor{green}{+3.00}  &
\textcolor{green}{+3.19}  &
\textcolor{green}{+2.55} \\
\bottomrule
\end{tabular}
\end{table}

We provide per-class AP for 3D object detection from the nuScenes validation set using BEVFusion in \Tabref{tab:bevfusion_compare}. From the results, we observe that, firstly, the improvements for large objects are significant, for example, buses, trailers, and construction vehicles. Secondly, objects with less diverse appearances, such as traffic cones and barriers, show more improvement, especially compared to trucks.
Thirdly, we note that the improvement is marginal for cars, while significant for pedestrians, motorcycles, and bicycles. This may be because the baseline already performs well for cars.
For pedestrians, motorcycles, and bicycles, even though distant objects from the ego car are generated less faithfully, \methodname can synthesize high-quality objects near the ego car, as shown in \Figref{fig:more2}-\ref{fig:more3}.
Therefore, more accurate detection of objects near the ego car contributes to improvements for these classes.
Overall, mAP improvement comes with promotion in all classes' AP, indicating \methodname can indeed help the training of perception models.

\section{More results for BEV segmentation}
BEVFusion is also capable of BEV segmentation and considers most of the classes we used in the BEV map condition. Due to the lack of baselines, we present the results in \Tabref{tab:bevfusion_seg} to facilitate comparison for future works.
As can be seen, the 272$\times$736 resolution does not outperform the 224$\times$400 resolution.
This is consistent with the results from CVT in \Tabref{tab:test} on the Road segment. Such results confirm that better map controls rely on maintaining the original aspect ratio for generation training (\ie, avoiding cropping on each side).
\begin{table}[h]
\vspace{-0.3cm}
\centering
\caption{Generation fidelity to BEV map conditions. Results are tested with BEVFusion for BEV segmentation on the nuScenes validation set.}
\label{tab:bevfusion_seg}
\begin{tabular}{@{}l|c|cc@{}}
\toprule
\multirow{2.5}{*}{Methods} & \multirow{2.5}{*}{resolution} & \multicolumn{2}{c}{mIOU for 6 classes} \\\cmidrule(l){3-4} 
            &                & CAM-only & CAM+LiDAR \\
\midrule
Oracle      & -              & 57.09    & 62.94     \\
Oracle      & 224$\times$400 & 52.72    & 58.49     \\
\midrule
\methodname              & 224$\times$400              & \textbf{30.24}     & \textbf{48.21}    \\
\methodname & 272$\times$736 & 28.71    & 47.12     \\ \bottomrule
\end{tabular}
\vspace{-0.3cm}
\end{table}

\section{Generalization of Camera Parameters}
To improve generalization ability, \methodname encodes raw camera intrinsic and extrinsic parameters for different perspectives. 
However, the generalization ability is somewhat limited due to nuScenes fixing camera poses for different scenes.
Nevertheless, we attempt to exchange the intrinsic and extrinsic parameters between the three front cameras and three back cameras.
The comparison is shown in \Figref{fig:cam-generalize}.
Since the positions of the nuScenes cameras are not symmetrical from front to back, and the back camera has a 120$^{\circ}$ FOV compared to the 70$^{\circ}$ FOV of the other cameras, clear differences between front and back views can be observed for the same 3D coordinates.
\begin{figure}[h]
    \vspace{-0.4cm}
    \centering
    \includegraphics[width=\linewidth]{figure/cam_generalize.pdf}
    \caption{
    To show the generalization ability of learned camera encoding, we exchange the camera parameters between 3 front cameras and 3 back cameras. The 3D position is the same for two generations. We highlight some areas (with box boxes)}
    \label{fig:cam-generalize}
\end{figure}

\newpage
\section{More Generation Results}
We show some corner-case~\citep{li2022coda} generations in \Figref{fig:hard}, and more generations 
in \Figref{fig:more1}-\Figref{fig:more3}.

\begin{figure}[h]
    \centering
    \includegraphics[width=0.98\linewidth]{more_visual/v2_7_final2.png}
    \includegraphics[width=0.98\linewidth]{more_visual/v2_0_final1.png}
    \includegraphics[width=0.98\linewidth]{more_visual/v2_3_final1.png}
    \caption{{Generation from \methodname with corner-case annotations}.
    }
    \label{fig:hard}
\end{figure}
    
\begin{figure}[ht]
    \centering
    \includegraphics[width=0.98\linewidth]{more_visual/3_final1.png}
    \includegraphics[width=0.98\linewidth]{more_visual/4_final2.png}
    \includegraphics[width=0.98\linewidth]{more_visual/5_final1.png}

    \caption{{Generation from \methodname with annotations from nuScenes validation set.}}
    \label{fig:more1}
\end{figure}

\begin{figure}[ht]
    \centering
    \includegraphics[width=0.98\linewidth]{more_visual/7_final1.png}
    \includegraphics[width=0.98\linewidth]{more_visual/14_final2.png}
    \includegraphics[width=0.98\linewidth]{more_visual/v2_1_final3.png}

    \caption{{Generation from \methodname with annotations from nuScenes validation set.}}
    \label{fig:more2}
\end{figure}

\begin{figure}[ht]
    \centering
    \includegraphics[width=0.98\linewidth]{more_visual/v2_4_final3.png}
    \includegraphics[width=0.98\linewidth]{more_visual/v2_5_final3.png}
    \includegraphics[width=0.98\linewidth]{more_visual/v2_6_final0.png}
    \caption{{Generation from \methodname with annotations from nuScenes validation set.}}
    \label{fig:more3}
\end{figure}
